# Supplementary material for: A New Statistical Model of Electroencephalogram Noise Spectra for Real-time Brain-Computer Interfaces
Source: arXiv:1608.03464 source file (2016-07-24)
Supplement: Supplementary file 4 [file 2_ROC.tex]

{\color{\AzadehColor}
\subsection{Comparison and Validation Metrics for SSVEP Algorithms}\label{subsec:ROC}

	The following section presents a preview of an innovative, statististically sound, and extremely flexible methodology we developed specifically for the comparison and validation of SSVEP algorithms. It forms the foundation for the single-trial receiver operating characterstics (ROC) graph of \myfig{fig:SNRTab_ROC} and \myfig{fig:LM_ROC} and the summary statistics of \mytable{tab:SNR_vs_GVZM_summary} and \mytable{tab:LM_vs_GVZM_summary}. The details will be published separately.


} % color
