# Supplementary material for: A New Statistical Model of Electroencephalogram Noise Spectra for Real-time Brain-Computer Interfaces
Source: arXiv:1608.03464 source file (2016-07-24)
Supplement: Supplementary file 5 [file 3_ROC_protocol.tex]

{\color{\AzadehColor}

	\myskip{\tny}
	\textbf{SSVEP Estimation Protocol}
	\myskip{\tny}

	Let $\mathbf{S}\Paren{\tau}$ be the signal from a randomly-selected instance $\tau$ of an SSVEP experiment. We refer to $\tau$ as a ``trial.'' The signal may be the actual raw EEG time series, a processed EEG spectrum, or even an arbitrary index into a table of signal exemplars. What is important is that  $\mathbf{S}\Paren{\tau}$ must be an \myemph{observable} random variable of the \myemph{unobservable} trial instance $\tau$ which ranges over the underlying probability space $\Paren{\mathrm{T},P}$ governing the experiment. That is, each trial $\tau \in \mathrm{T}$, whose probability of occurrence is $P\Paren{\tau}$, encapsulates all the uncertainties of the SSVEP experiment: 
\begin{itemize}
	\item Variations between subjects chosen at random.
	\item Variations within the same subject on different days, different times of the same day, or different moods.
	\item Impedence variations caused by non-uniform application of electrode gel.
	\item Artifacts.
	\item Stray electromagnetic fields.
	\item The particular stimulus frequencies used for this trial.
	\item The stimulus frequency to which the subject attends as well as the time interval of attention.
	\item The dice-rolls or coin-tosses we may use for randomized decision rules.
	\item The vast number of other unnamed lurking variables in any SSVEP/EEG experiment.
\end{itemize}

	Let $F_\mathrm{ssvep}\Paren{\tau}$ be the (random) set of \myemph{stimulus frequencies} we are trying to estimate from $\mathbf{S}\Paren{\tau}$ during trial $\tau$. Note that $F_\mathrm{ssvep}\Paren{\tau}$ should include all possible fundamental stimulus frequencies which were flashing when $\mathbf{S}\Paren{\tau}$ was observed. It may also include some harmonics (\myfig{fig:chi2_8Hz}) and subharmonics \cite{herrmann-2001} of these fundamental SSVEP frequencies. 
	
	Let $F_{\mathrm{test} \undefsymb}$ be an initial set of \myemph{test frequencies}. When given any single-trial signal $\mathbf{S}$, our estimation protocol is to succesively test every $f \in F_{\mathrm{test} \undefsymb}$ for its presence or absence in $F_\mathrm{ssvep}\Paren{\tau}$. Thus we are performing \myemph{frequency estimation by \textit{m}-ary testing} \cite{levy-book-2008}, where \textit{m} is the size of $F_{\mathrm{test} \undefsymb}$. A given testing procedure may or may not have access to $F_\mathrm{ssvep}\Paren{\tau}$; that is, it may or may not be \myemph{blind}. 
	
	An essential aspect of SSVEP estimation, especially for BCI applications, is that every trial partitions $F_{\mathrm{test} \undefsymb}$ into three subsets: 
\begin{enumerate}
	\item Those $f$ satisfying $f \in F_{\mathrm{test} \undefsymb} \cap F_\mathrm{ssvep}\Paren{\tau}$.
	\item Those $f \in F_{\mathrm{test}\undefsymb} \setminus F_\mathrm{ssvep}\Paren{\tau}$ which thus were not present during this trial but \myemph{might have been}. These could be, for example, frequencies of non-selected fields during a BCI test. 
	\item All other $f \in F_{\mathrm{test}\undefsymb}$.
\end{enumerate}

	In typical blind SSVEP frequency estimation, case (3) vastly outnumbers (1) and (2). For example, the data used in \mysec{sec:SSVEP} contained 614 initial test frequencies while there were only 19 possible distinct stimulus frequencies and harmonics. In such a situation, simple \textit{m}-ary control procedures such as Bonferroni correction (see \cite{benjamini-hochberg-1995} for a survey) are out of the question because they yield impractically small corrected significance levels. Even less conservative procedures such as those used to control the false discovery rate (FDR) \cite{benjamini-krieger-yekutieli-2006} yield overall significance levels which often produce no discoveries at all. This because the signal-to-noise ratio of SSVEP signals is usually too low for estimation statistics to yield sufficiently small \textit{P}-values even at fundamental stimulus frequencies.
	
	Moreover, non-stimulus frequencies that we particularly want to reject may slip into the signal, the most important example being the frequencies of non-selected but still visible fields during BCI experiments. The assessment of any algorithm must test its ability to positively exclude these potential contaminants even when blind.
	
	 It is therefore essential to develop estimation and validation procedures which can distinguish the combined situation $(1) \cup (2)$ from (3). 
	
	A solution to all the problems of the preceeding paragraphs is to assume a second randomly-varying set $F_\textrm{null}\Paren{\tau}$ of \myemph{null frequencies} such that $F_\textrm{null}\Paren{\tau} \cap F_\textrm{ssvep}\Paren{\tau} = \emptyset$. Once the signal $\mathbf{S}\Paren{\tau}$ is observed, the hypotheses we decide at each test frequency $f \in F_{\mathrm{test} \undefsymb}$ are
	
\myskip{\tny}
\quadOne$\mathrm{H}_0\Paren{f}$: \; $f \in F_\textrm{null}\Paren{\tau}$

\quadOne$\mathrm{H}_\mathrm{alt}\Paren{f}$: $f \in F_\textrm{ssvep}\Paren{\tau}$
\myskip{\tny}

\noindent but we \myemph{do not assume} that the testing procedure always makes a decision between $\mathrm{H}_0\Paren{f}$ and $\mathrm{H}_\mathrm{alt}\Paren{f}$; that is, we must allow \myemph{undetermined} as a possibility.
	
	We require a \myemph{ground truth frequency estimation algorithm} for SSVEP experiments as a baseline. This  may be:
\begin{itemize}
	\item A look-up table from a laboratory notebook.
	\item An electronic spectral analyzer or oscilloscope.
	\item Gold-standard spectral estimation software.
	\item A synthetic ground truth algorithm which simulates real SSVEP results. This can be used for validating a new algorithm. It is the ground truth used to produce the tables and figures of \mysec{sec:SSVEP}.
\end{itemize}
The ground truth may or may not be blind. 
	We want to measure the performance of a \myemph{comparison algorithm} (which is usually assumed to be blind) against this ground truth.
	
	Both the ground truth and comparison algorithms may involve randomized decision rules \cite{levy-book-2008}. However we make the assumption that the randomization procedures of the two algorithms are \myemph{independent given $\mathbf{S}$}. That is, once the signal outcome $\mathbf{S} = \mathbf{S}\Paren{\tau}$ is known, whatever $\tau$-dependent dice-rolls or coin-tosses each uses to make its decisions about $\mathrm{H}_0\Paren{f}$ and $\mathrm{H}_\mathrm{alt}\Paren{f}$ are statistically independent of one another. We also assume that any randomized rules of each individual algorithm are independent at distinct test frequencies, given $\mathbf{S}$. (This latter assumption actually excludes some interesting potential algorithms but is required for the calculation of the parametrized contingency tables discussed below. However it is sufficiently general to hold for most practical algorithms including those from \mysec{sec:SSVEP}.)
	
	
} % color
