# Supplementary material for: A New Statistical Model of Electroencephalogram Noise Spectra for Real-time Brain-Computer Interfaces
Source: arXiv:1608.03464 source file (2016-07-24)
Supplement: Supplementary file 6 [file 4_ROC_CTstat.tex]

{\color{\AzadehColor}

	\myskip{\tny}
	\textbf{The Contigency Table Statistics}
	\myskip{\tny}

	 Since we do not assume that the two algorithm always determine the truth values of the two hypotheses, there are 9 possible outcomes for a test at $f \in F_{\mathrm{test} \undefsymb}$. The full $3 \times 3$ contingency table at $f$ is defined by \mytable{tab:CT_full}:
\input{\TabsDir/CT_3x3.tex}

	The 4 core cells are $0,1$-valued indicator functions given by:
	
\mybegeq{eq:CTcore}
\left\{
\begin{aligned}
\mathrm{TP}_\undefsymb\Paren{f} &= \Id_\mathrm{P}\Paren{f} \cdot \Id_\mathrm{alt}\Paren{f} \\
\mathrm{FP}_\undefsymb\Paren{f} &= \Id_\mathrm{P}\Paren{f} \cdot \Id_\mathrm{0}\Paren{f} \\
\mathrm{FN}_\undefsymb\Paren{f} &= \Id_\mathrm{N}\Paren{f} \cdot \Id_\mathrm{alt}\Paren{f} \\
\mathrm{TN}_\undefsymb\Paren{f} &= \Id_\mathrm{N}\Paren{f} \cdot \Id_\mathrm{0}\Paren{f},
\end{aligned} 
\right.
\myendeq
where $\Id_\mathrm{P}\Paren{f}$, $\Id_\mathrm{N}\Paren{f}$ are the indicators for accepting $\mathrm{H}_\mathrm{alt}\Paren{f}$, $\mathrm{H}_0\Paren{f}$ and $\Id_\mathrm{alt}\Paren{f}$, $\Id_\mathrm{0}\Paren{f}$ are the indicators for ground truth.

	The remaining labeled cells are fractional indicators whose values are in the interval $\Brack{0,1}$. They are used to compress the $3 \times 3$ table into a $2 \times 2$ table by allocating the indeterminate cells as described below:
	
	If no decision was reached by the comparison algorithm on a test frequency but its ground truth was determinable then we should regard that test as false. The logic is that sufficient information was available to the ground truth procedure but the comparison algorithm failed to extract it. These are the cells labeled $\mathrm{Fn}\Paren{f}$ and $\mathrm{Fp}\Paren{f}$ in \mytable{tab:CT_full}.
	
	If both the comparison and the ground truth algorithms were unable to determine the status of a frequency, then it should be excluded from both the initial set $F_{\mathrm{test} \undefsymb}$ of test  frequencies and any further analysis since neither algorithm is able to make any definitive statement about it. This is the blank cell in \mytable{tab:CT_full}. The resulting set of frequencies, at which at least one algorithm was determined, is denoted $F_\mathrm{test}$. In practice, $F_\mathrm{test}$ is usually much smaller than than $F_{\mathrm{test} \undefsymb}$. For example, in \mysec{subsec:SNR}, the 614 initial test frequencies are usually reduced to a few 10's. This balances the contingency counts, eliminating most of the problems discussed above in regards to Bonferroni and the FDR.
	
	The ambiguous situation is that in which the comparison algorithm arrived at a decision but no ground truth was available. We resolve this ambiguity by selecting a \myemph{null hypothesis bias} $\beta_0$, $0 \myle \beta_0 \myle 1$, which specifies how much the protocol favors $\mathrm{H}_0$ when ground truth is unknown. Using a legal metaphor, $\beta_0 = 1$ means that uncertain evidence always favors the defendant while $\beta_0 = 0$ means evidence of uncertain merit is nevertheless considered incriminating. This allows the unambigous assigment of the $\textrm{H}_\undefsymb$ cells as follows:
\mybegeq{eq:undefCT}
\left\{
\begin{aligned}
\mathrm{tP}\Paren{f} &= \Paren{1-\beta_0}\cdot\textrm{H}_\undefsymb \textrm{P}\Paren{f} \\
\mathrm{fP}\Paren{f} &= \beta_0\cdot\textrm{H}_\undefsymb \textrm{P}\Paren{f} \\
\mathrm{tN}\Paren{f} &= \Paren{1-\beta_0}\cdot\textrm{H}_\undefsymb \textrm{N}\Paren{f} \\
\mathrm{fN}\Paren{f} &= \beta_0\cdot\textrm{H}_\undefsymb \textrm{N} \Paren{f},
\end{aligned} 
\right.
\myendeq
where $\textrm{H}_\undefsymb \textrm{P}\Paren{f}$, $\textrm{H}_\undefsymb \textrm{N}\Paren{f}$ are the indicators for positive and negative decisions respectively under the condition that the ground truth for the test frequency $f$ is undetermined:
\[
\left\{
\begin{aligned}
\textrm{H}_\undefsymb \textrm{P}\Paren{f} &= \Id_\mathrm{P}\Paren{f} \cdot \Id_{\mathrm{H}\undefsymb}\Paren{f} \\
\textrm{H}_\undefsymb \textrm{N}\Paren{f} &= \Id_\mathrm{P}\Paren{f} \cdot \Id_{\mathrm{H}\undefsymb}\Paren{f}.
\end{aligned} 
\right.
\]


Note that these are typically fractional indicators.

	The marginal cells $\mathrm{P}_\undefsymb\Paren{f}$, $\mathrm{N}_\undefsymb\Paren{f}$, $\mathrm{m}_{\mathrm{alt} \undefsymb}\Paren{f}$, $\mathrm{m}_{0 \undefsymb}\Paren{f}$, and $\mathrm{m}\Paren{f}$ are the sums of the associated columns and rows.
	
	The derived $2 \times 2$ table now is given by \mytable{tab:CT_derived} with cells
\mybegeq{eq:defCT}
\left\{
\begin{aligned}
\mathrm{TP}\Paren{f} &=  \mathrm{TP}_\undefsymb\Paren{f} + \mathrm{tP}\Paren{f} \\
\mathrm{FP}\Paren{f} &= \mathrm{FP}_\undefsymb\Paren{f} + \mathrm{fP}\Paren{f} + \mathrm{Fp}\Paren{f} \\
\mathrm{FN}\Paren{f} &= \mathrm{FN}_\undefsymb\Paren{f} + \mathrm{Fn}\Paren{f} + \mathrm{fN}\Paren{f} \\
\mathrm{TN}\Paren{f} &=  \mathrm{TN}_\undefsymb\Paren{f} + \mathrm{tN}\Paren{f}
\end{aligned} 
\right.
\myendeq
and marginals as shown.
\input{\TabsDir/CT_2x2.tex}

\mybegdef{def:CT_0} The (unparameterized) \myemph{contingency table statistic} is defined to be
\[
	\Op{CT}\Paren{\mathbf{S}} \Eqdef \sum\limits_{f \in F_\mathrm{test}} {\Op{CT}\Paren{f,\mathbf{S}}},
\]
where $\Op{CT}\Paren{f,\mathbf{S}}$ denotes the derived $2 \times 2$ table at $f$ given by \mytable{tab:CT_derived} when processing signal $\mathbf{S}$ .
\myenddef

	Note that because we have allowed randomized decision rules, $\Op{CT}\Paren{\mathbf{S}}$ is actually a multi-dimensional random variable on the underlying probability space of the collection of trials, not merely a function of $\mathbf{S}$. It is this statistic which we use to make inferences about the the relative performance of a comparison algorithm to ground truth.
	
	Generally the comparison algorithm works by computing the \textit{P}-value of some spectral statistic (e.g, the SNR (\mydef{def:SNR}) or the Liavas, et al. spectral \textit{F}-ratio \myeq{eq:F-stat}, with or without the GVZM baseline) at each $f \in F_\mathrm{test}$ and comparing it to some preassigned significance level $\alpha$.
	
	It is also extremely helpful to be able to vary the frequency precision of each algorithm's decisions. Let $r > 0$ be a frequency radius in Hz. Define the \myemph{parametrized hypotheses} at $f \in F_\mathrm{test}$ to be 
	
\myskip{\tny}
\quadOne$\mathrm{H}_0\Paren{\alpha,r;f}$: \; $\Paren{\forall g}$ $\Abs{g-f} < r$ implies $g \notin F_\mathrm{stim}$

\quadOne$\mathrm{H}_\mathrm{alt}\Paren{\alpha,r;f}$: $\Paren{\exists g}$ $\Abs{g-f} < r$ and $g \in F_\mathrm{stim}$,
\myskip{\tny}

\noindent where the membership of $g$ in or out of $F_\mathrm{stim}$ is determined at significance level $\alpha$.

\mybegdef{def:CT} The (parameterized) \myemph{contingency table statistic} is defined to be
\[
	\Op{CT}\Paren{\alpha,r} \Eqdef \sum\limits_{f \in F_\mathrm{test}} {\Op{CT}\Paren{\alpha,r;f}},
\]
\myenddef
\noindent where the table at $f$ is determined by testing $\mathrm{H}_0\Paren{\alpha,r;f}$ and $\mathrm{H}_\mathrm{alt}\Paren{\alpha,r;f}$.

	Again, $\Op{CT}\Paren{\alpha,r}$ is a multi-dimensional random variable. The parameters $\alpha,r$ can be altered to examine the relative performance of the comparison algorithm at various \myemph{operating points} \cite{fawcett-2006}.


} % color
