# Supplementary material for: A New Statistical Model of Electroencephalogram Noise Spectra for Real-time Brain-Computer Interfaces
Source: arXiv:1608.03464 source file (2016-07-24)
Supplement: Supplementary file 7 [file 5_ROC_CTestimator.tex]

{\color{\AzadehColor}

	\myskip{\tny}
	\textbf{The Optimal Estimator Metric}
	\myskip{\tny}

} % color
